# Supplementary material for: Ab-initio simulations and measurements of the free-free opacity in Aluminum
Source: arXiv:1806.02726 source file (2018-06-07)
Supplement: Supplementary file 1 [file SupplementaryMaterial.pdf]

## SUPPLEMENTARY MATERIAL

The experiment was performed at the Artemis facility for ultrafast XUV science, part of the Central Laser facility at the Rutherford-Appleton Laboratory, UK. This is a 1kHz repetition rate beamline that provides standard methods to filter out the IR from the HHG pulses, and a high-resolution monochromator to select individual harmonics with minimal pulse stretching. The transmission was measured using a micro-channel plate (MCP) detector, the optical output of which was imaged onto a CCD. The linearity of the optical system was verified during the experiment across the entire dynamic range of transmitted signals and for all exposure time durations. Typical exposure times ranged from 1-5 seconds, so the data integrates over several thousand shots for each data point. We provide here some additional details on the data processing and error calculation.

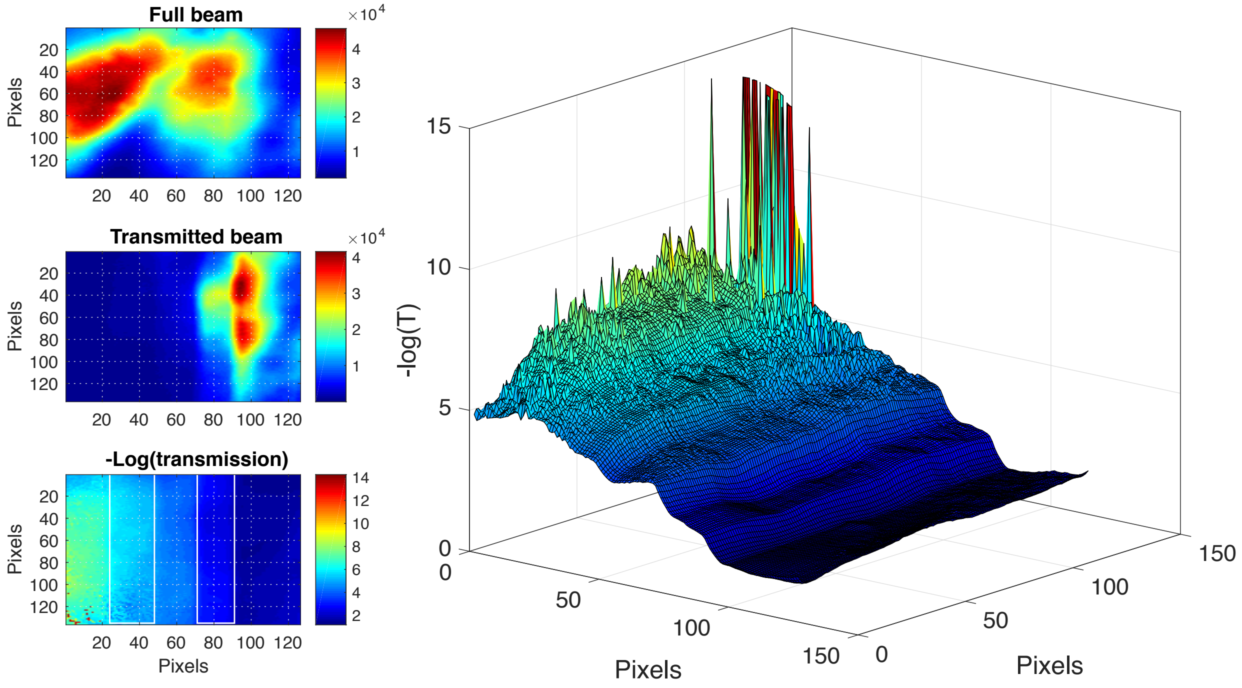


FIG. 1. Measurement of the transmission through the Al step target for the 15th laser harmonic at around 24 eV. The left panels show the spatial intensity distribution of the HHG beam without a target (full beam), transmitted through the step target, and the negative log of the ratio of the two yielding the total transmission. The last panel is also shown on the right in 3D to illustrate that the steps of the target are clearly visible in the absorption measurement.

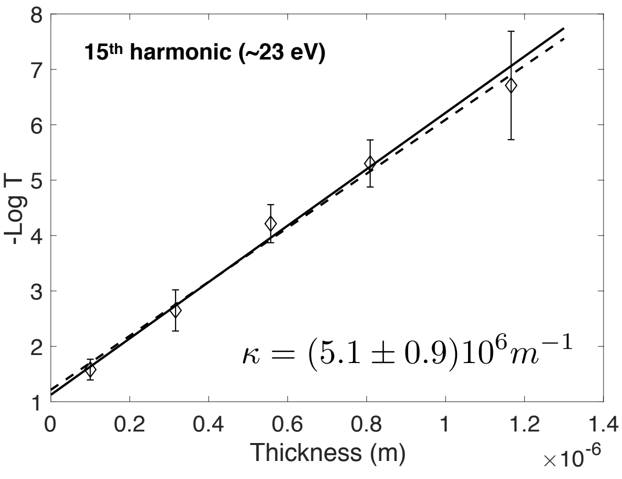


FIG. 2. Observed transmission of the 15th harmonic through the Al step target sample. Following Eq. 2 we perform a linear fit to the five data points to extract $\kappa(\omega)$ (the slope), $\alpha(\omega)$ (the y-intercept), and related errors.

The transmission $T$ of the VUV pulse is given by the Beer–Lambert law as:

$$T = \exp(-\kappa(\omega)d - \alpha(\omega)), \tag{1}$$

where $\kappa(\omega)$ is the frequency-dependent absorption coefficient of Al, $d$ is the variable thickness of the Al sample, and $\alpha$ is the attenuation contribution from absorption in oxide layers and other contaminants, assumed to give the same contribution to all regions of the target. By taking the negative logarithm of the transmission we can write a linear equation for the absorption coefficients as a function of the variable $d$, the thicknesses of the Al step target:

$$-\log(T) = \kappa(\omega)d - \alpha(\omega). \tag{2}$$

We show the measured attenuation through the sample in Fig. 1 for the 15th laser harmonic. The steps can easily be observed in the 3D plot of the transmission. Because the sample thickness is accurately known before the experiment, we can extract experimental values for both $\kappa(\omega)$ and $\alpha(\omega)$ by fitting the data using the linear function of sample thickness given in Eq. 2. We show this procedure in Fig. 2. We find $\kappa(\omega) = 5.1 \times 10^6$ m$^{-1}$, with an uncertainty of $0.9 \times 10^6$ m$^{-1}$, where we quote a 95% confidence interval, i.e. $\pm 2\sigma$. The same procedure was repeated for all the harmonics (11-37) to yield the data shown in Fig. 2(a) of the main paper.
